# Supplementary material for: Distances, Luminosities, and Temperatures of the Coldest Known Substellar Objects
Source: arXiv:1309.1422 source file (2013-09-05)
Supplement: Supplementary file 1 [file Science_Supplementary_Materials_Word_template.pdf]

This is the *Science* template for presenting and formatting your Supplementary Materials. To organize your Supplementary Materials section, please follow the instructions below. Once formatted, you should delete this first page of instructions. This template is designed to provide an indexed/bookmarked PDF file that will help readers navigate to sections or specific figures or tables. To ensure proper indexing, please maintain the Word styles in the template or reapply them afterward.

### **Overview:**

Supplementary Materials present additional information in support of the conclusions of your paper, such as a description of the materials and methods, controls, or tabulated data presented in graphs or figures in the paper. It will generally consist of one integrated PDF file. Audio or movie files or large data tables can be presented as separate files. Further information is available [here](#).

This section should not be used for additional discussion, analysis, or interpretations. It is not to be used as a forum to critique other publications.

References can be cited in the supplementary text section. These should be cited in order following the references in the main text as per *Science* style (italicized number in parentheses). One full reference list should be provided for all of the cited references at the end of the main paper.

### **Using the Template**

Paste the appropriate text (title, author list and corresponding authors into the cover page). Keep our original formatting, or reapply the appropriate styles after pasting. There are three Word paragraph styles: SM Heading (to be applied to Major heads including Figure and Table labels), SM Subheading (to be applied to subheads), and SOM text (for text, equations, etc.) and SM captions (for figure or table captions)

On the cover page, complete the relevant description of the SM (by deleting text that does not apply).

Copy and paste relevant text into each appropriate section of the template. Keep the formatting of this template, or restyle paragraphs as indicated. Each figure should be on a separate page and can be placed above each caption. To add additional captions, simply copy and paste (repeatedly) the last caption template. Large tables that extend beyond the width of the page should be provided as separate files.

Large amounts of text can be grouped by subheads. To repeat subheads, simply copy the subhead and reapeat/rename. To add more figures, copy and paste to repeat the styled dummy text for more figure or table captions.

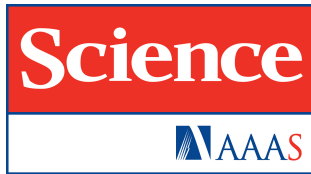

## Supplementary Materials for

### Distances, Luminosities, and Temperatures of the Coldest Known Substellar Objects

Trent J. Dupuy<sup>1,2</sup> and Adam L. Kraus<sup>1,3</sup>

<sup>1</sup>Harvard-Smithsonian Center for Astrophysics, 60 Garden St, Cambridge, MA 02138, USA

<sup>2</sup>Hubble Fellow

<sup>3</sup>Astronomy Department, University of Texas at Austin, 1 University Station C1400, Austin, TX 78712, USA

correspondence to: [tdupuy@cfa.harvard.edu](mailto:tdupuy@cfa.harvard.edu)

#### **This PDF file includes:**

Materials and Methods  
Supplementary Text  
Figures S1 to S5  
Tables S1 to S6

## **Materials and Methods**

### Subhead

Type or paste text here. Maintain formatting or style as “SM text.” You can break this section up into subheads as needed (e.g., one on “Materials” and one on “Methods”)

## **Supplementary Text**

### Subhead

Type or paste text here. This should be additional explanatory text, such as: extended technical descriptions of results, full details of mathematical models, extended lists of acknowledgements etc. It should not be additional discussion, analysis, interpretation or critique. Keep this formatting or style as SM text.

<insert page break then Fig S1 here>

### **Fig. S1.**

Type or paste caption here. Maintain formatting or style as “SM caption.” Create a page break and paste in the figure above the caption.

<insert page break then Fig S2 here>

### **Fig. S2**

Type or paste caption here. Maintain formatting or style as “SOM caption.” Create a page break and paste in the figure above the caption.

<insert page break then Fig S3 here>

### **Fig. S3**

Type or paste caption here. Maintain formatting or style as “SM caption.” Create a page break and paste in the figure above the caption.

<insert page break here>

### **Table S1.**

Type or paste caption here. Maintain formatting or style as “SM caption.”

<insert Table S1 here followed by a page break >

### **Table S2.**

Type or paste caption here. Maintain formatting or style as “SM caption.”

<insert Table S1 here followed by a page break >

**Movie S1**

Type or paste caption here. Maintain formatting or style as “SM caption.”

**Audio S1**

Type or paste caption here. Maintain formatting or style as “SM caption.”

**Additional Data table S1 (separate file)**

Type or paste caption here. Maintain formatting or style as “SM caption.”
